# Supplementary material for: Weak-coupling to strong-coupling quantum criticality crossover in a Kitaev quantum spin liquid $\alpha$-RuCl$_3$
Source: arXiv:2203.13407 ancillary file (2022-03-25)
Supplement: Supplementary file 1 [file Supplementary.pdf]

Supplemental Material for

**Weak-coupling to strong-coupling quantum criticality crossover  
in a Kitaev quantum spin liquid  $\alpha$ -RuCl<sub>3</sub>**

Jae-Ho Han<sup>\*</sup>, Seung-Hwan Do<sup>\*</sup>, Kwang-Yong Choi, Sang-Youn Park, Jae-You Kim, Sungdae Ji<sup>†</sup>, Ki-Seok Kim<sup>‡</sup>, and Jae-Hoon Park<sup>§</sup>

<sup>\*</sup> These authors contributed equally to this work

<sup>†</sup> [jsungdae@kaeri.re.kr](mailto:jsungdae@kaeri.re.kr)

<sup>‡</sup> [tkfkd@postech.ac.kr](mailto:tkfkd@postech.ac.kr)

<sup>§</sup> [jhp@postech.ac.kr](mailto:jhp@postech.ac.kr)

# Table of Contents

|                                                                                                                                                                                |           |
|--------------------------------------------------------------------------------------------------------------------------------------------------------------------------------|-----------|
| <b>A. Effective field theory, renormalization group analysis, and dynamic spin susceptibility for the high-energy weak-coupling fixed point.....</b>                           | <b>3</b>  |
| 1. Construction of an effective field theory.....                                                                                                                              | 3         |
| 2. Wilsonian renormalization group analysis.....                                                                                                                               | 6         |
| 3. Dynamic spin susceptibility.....                                                                                                                                            | 11        |
| <br><b>B. Effective field theory, dynamic spin susceptibility, specific heat, and dynamical mean-field theory analysis for the low-energy strong-coupling fixed point.....</b> | <b>13</b> |
| 1. Effective field theory, dynamic spin susceptibility, and specific heat for the local quantum criticality.....                                                               | 13        |
| 2. Dynamical mean-field theory analysis for the low-energy strong-coupling fixed point.....                                                                                    | 15        |
| <br><b>Appendix.....</b>                                                                                                                                                       | <b>18</b> |
| A. Self-energy and vertex corrections.....                                                                                                                                     | 18        |
| B. Dynamic spin susceptibility.....                                                                                                                                            | 20        |
| <br><b>References and Notes.....</b>                                                                                                                                           | <b>23</b> |

## A. Effective field theory, renormalization group analysis, and dynamic spin susceptibility for the high-energy weak-coupling fixed point

### 1. Construction of an effective field theory

In order to construct an effective field theory, we start from a ferromagnetic Kitaev Hamiltonian (1)

$$\begin{aligned} H_K &= -K_x \sum_{x\text{-bond}} \sigma_i^x \sigma_j^x - K_y \sum_{y\text{-bond}} \sigma_i^y \sigma_j^y - K_z \sum_{z\text{-bond}} \sigma_i^z \sigma_j^z \\ &= -K_x \sum_r \sigma_{r,w}^x \sigma_{r+x,b}^x - K_y \sum_r \sigma_{r+y,b}^y \sigma_{r,w}^y - K_z \sum_r \sigma_{r,b}^z \sigma_{r,w}^z, \end{aligned} \quad (\text{S1})$$

Here local spins satisfy the commutation relation  $[\sigma_i^\alpha, \sigma_j^\beta] = 2i\epsilon_{\alpha\beta\gamma}\sigma_i^\gamma\delta_{ij}$ . The lattice vector is given by  $r = n_x a_x + n_y a_y$  with  $n_x, n_y \in \mathbb{Z}$ , where the lattice unit cell is spanned by  $a_x = a(\sqrt{3}/2, 3/2)$  and  $a_y = a(-\sqrt{3}/2, 3/2)$  for the hexagonal bond length  $a$ . The subscripts “w” and “b” represent two triangular sublattices as shown in Fig. S1A (white and black filled circles).

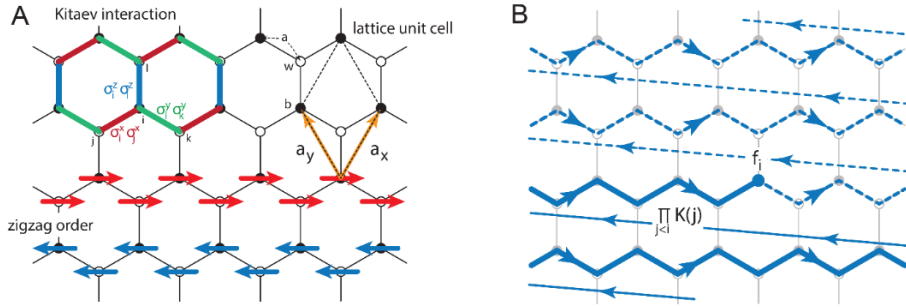

**Fig. S1 Schematic figure of the model.** (A) Honeycomb lattice, Kitaev interaction, zigzag antiferromagnetic order, lattice and basis, and lattice unit cell. (B) Order of lattice points.

Now we introduce zigzag AFM ordering observed below  $T_N$  in  $\alpha$ -RuCl<sub>3</sub> as shown in Fig. S1A (2-5). This AFM order likely results from the interplay among Kitaev, Heisenberg, and anisotropic spin exchange interactions on the honeycomb lattice. Here, we implement a zigzag AFM fixed point in the Kitaev spin liquid state and investigate emergent physics near this conjectured fixed point. The corresponding effective Hamiltonian, which represents the coupling between the zigzag AFM fluctuation and Kitaev spins, can be given by

$$H_{ZZ} = -g \sum_i \phi_i \sigma_i^z, \quad (\text{S2})$$

where  $\phi_i = \langle \sigma_i^z \rangle$  and  $g$  is an effective coupling constant. In the zigzag AFM phase,  $\phi_i$  become finite with  $\phi_{r,w} = -\phi_{r,b}$ .

6, 7)

$$\sigma_i^z = 2f_i^\dagger f_i - 1, \quad \sigma_i^- = \frac{1}{2}(\sigma_i^x + i\sigma_i^y) = \left( \prod_{j<i} K(j) \right) f_i^\dagger, \quad \sigma_i^+ = \frac{1}{2}(\sigma_i^x - i\sigma_i^y) = \left( \prod_{j<i} K(j) \right) f_i, \quad (\text{S3})$$

where  $K(j) = 2f_j^\dagger f_j - 1$  and the order of lattice points is shown in Fig. S1B. Here, the spinless fermion field represents a domain wall excitation, where the nonlocal string operator implies a topological defect (8). It is straightforward to check out  $[\sigma_i^z, \sigma_j^\pm] = \pm 2\sigma_i^\pm \delta_{ij}$ ,  $[\sigma_i^+, \sigma_j^-] = \sigma_i^z \delta_{ij}$  for spin operators and  $\{f_i^\dagger, f_j\} = \delta_{ij}$ ,

$\{f_i, f_j\} = \{f_i^\dagger, f_j^\dagger\} = 0$  for the JW fermions. This nonlocal transformation makes us to rewrite Kitaev and AFM Ising spin interaction terms as follows;

$$H_K = -K_x \sum_r (f_{r+x,b}^\dagger + f_{r+x,b})(f_{r,w}^\dagger - f_{r,w}) - K_y \sum_r (f_{r+y,b}^\dagger + f_{r+y,b})(f_{r,w}^\dagger - f_{r,w}) - K_z \sum_r (2f_{r,b}^\dagger f_{r,b} - 1)(2f_{r,w}^\dagger f_{r,w} - 1), \quad (S4)$$

$$H_{ZZ} = -g \sum_r [\phi_{r,w}(2f_{r,w}^\dagger f_{r,w} - 1) + \phi_{r,b}(2f_{r,b}^\dagger f_{r,b} - 1)]. \quad (S5)$$

The Kitaev Hamiltonian can be diagonalized by introducing two complex fermions, which correspond to mixtures of fermions on two sites (black and white) linked by the directional  $z$ -bond in Fig. S1A, defined as (6)

$$\chi_r = \text{Re}f_{r,w} - i\text{Im}f_{r,b}, \quad \psi_r = \text{Im}f_{r,w} + i\text{Re}f_{r,b}. \quad (S6)$$

Then the Kitaev and coupling Hamiltonians are presented by

$$H_K = -K_x \sum_r (\psi_{r+x}^\dagger - \psi_{r+x})(\psi_r^\dagger + \psi_r) - K_y \sum_r (\psi_{r+y}^\dagger - \psi_{r+y})(\psi_r^\dagger + \psi_r) + K_z \sum_r (2\chi_r^\dagger \chi_r - 1)(2\psi_r^\dagger \psi_r - 1), \quad (S7)$$

$$H_{ZZ} = -ig \sum_r \phi_r (\psi_r^\dagger \chi_r^\dagger + \psi_r \chi_r), \quad (S8)$$

where we set  $\phi_{r,w} = -\phi_{r,b} \equiv \phi_r/2$ . Here  $\chi_r^\dagger \chi_r$  can be recognized to be a conserved quantity, i.e.  $[\chi_r^\dagger \chi_r, H_K] = 0$ , in the absence of zigzag AFM fluctuations. This conservation identifies  $\chi_r^\dagger \chi_r$  with the  $Z_2$  flux density, described by localized Majorana fermions in the original Kitaev model. As a result, the ground state of the Kitaev Hamiltonian is described by  $\chi_r^\dagger \chi_r = 0$ . Within this sector, the Kitaev Hamiltonian becomes reduced into a same form as the  $p$ -wave superconductivity of chargeless spinons

$$H_K = -K_x \sum_r (\psi_{r+x}^\dagger - \psi_{r+x})(\psi_r^\dagger + \psi_r) - K_y \sum_r (\psi_{r+y}^\dagger - \psi_{r+y})(\psi_r^\dagger + \psi_r) - K_z \sum_r (2\psi_r^\dagger \psi_r - 1) = \sum_k \epsilon_k \psi_k^\dagger \psi_k + \sum_k \frac{i\Delta_k}{2} (\psi_k^\dagger \psi_{-k}^\dagger + \psi_k \psi_{-k}). \quad (S9)$$

Here, the energy dispersion relation is given by  $\epsilon_k = -2K_z - 2K_x \cos k \cdot a_x - 2K_y \cos k \cdot a_y$  and the  $p$ -wave pairing amplitude becomes  $\Delta_k = 2K_x \sin k \cdot a_x + 2K_y \sin k \cdot a_y$ , where both  $a_x$  and  $a_y$  span the lattice unit cell as discussed before.  $\psi_k$  is the Fourier transform of  $\psi_r$ -field given by  $\psi_r = \frac{1}{\sqrt{N_z}} \sum_k e^{ik \cdot r} \psi_k$ , where  $N_z$  is the number of  $z$ -bonds or the number of triangular Bravais lattice sites in the honeycomb lattice.

Performing the Bogoliubov transformation of  $\gamma_k = u_k \psi_k + v_k \psi_{-k}^\dagger$ , where the coherence factors of  $u_{-k} = u_k$  and  $v_{-k} = -v_k$  satisfy  $|u_k|^2 + |v_k|^2 = 1$ , we found that the quasiparticle spectrum is given by  $E_k = \sqrt{\epsilon_k^2 + \Delta_k^2}$ . (13) It turns out that gapless points arise at  $k = \pm k_0$  with  $k_0 = \frac{1}{3}b_x - \frac{1}{3}b_y$  in the symmetric case of  $K_x = K_y = K_z \equiv K$ , where the reciprocal lattice vectors are given by  $b_x = 2\pi a(1/\sqrt{3}, 1/3)$ ,  $b_y = 2\pi a(-1/\sqrt{3}, 1/3)$ . See Fig. S2.

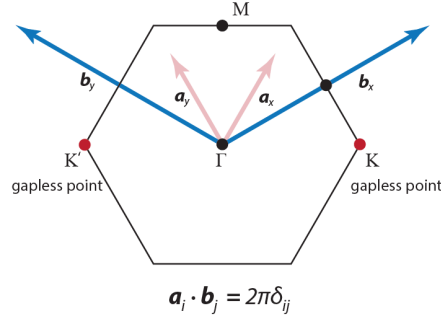

**Fig. S2 Brillouin zone and gapless points.** The red points shows two gapless points  $K$  ( $\mathbf{k} = \mathbf{k}_0$ ) and  $K'$  ( $\mathbf{k} = -\mathbf{k}_0$ ) in the Brillouin zone.

Taking into account zigzag AFM fluctuations described by  $\phi_r$ ,  $\chi_r^\dagger \chi_r$  is not a conserved quantity any more. Hereafter, we only consider the symmetric case,  $K_x = K_y = K_z \equiv K$ , and the effective Hamiltonians become

$$H_K = \sum_k \epsilon_k \psi_k^\dagger \psi_k + \sum_k \frac{i\Delta_k}{2} (\psi_k^\dagger \psi_{-k}^\dagger + \psi_k \psi_{-k}) + 2K \sum_k \chi_k^\dagger \chi_k + \frac{4K}{N_z} \sum_{k,p,q} \chi_p^\dagger \chi_{p+q} \psi_{k+q}^\dagger \psi_k \quad (\text{S10})$$

$$H_{ZZ} = -ig \sum_{k,q} \phi_q (\chi_{-k+q}^\dagger \psi_k^\dagger + \psi_k \chi_{-k-q}), \quad (\text{S11})$$

where  $\chi_k$  and  $\phi_k$  are the Fourier transformations as  $\chi_r = \frac{1}{\sqrt{N_z}} \sum_k e^{ik \cdot r} \chi_k$  and  $\phi_r = \sum_k e^{ik \cdot r} \phi_k$ , and an irrelevant constant term is eliminated. We note that  $\phi_q^\dagger = \phi_{-q}$ , where  $\phi_r$  is real.

In order to construct an effective field theory, we consider low energy states near the gapless points and obtain

$$\begin{aligned} H_K = & \sum_k (\epsilon_{+,k} \psi_{+,k}^\dagger \psi_{+,k} + \epsilon_{-,k} \psi_{-,k}^\dagger \psi_{-,k}) \\ & + \sum_k \left\{ \frac{i\Delta_{+,k}}{2} (\psi_{+,k}^\dagger \psi_{-,-k}^\dagger + \psi_{+,k} \psi_{-,-k}) + \frac{i\Delta_{-,k}}{2} (\psi_{-,k}^\dagger \psi_{+,-k}^\dagger + \psi_{-,k} \psi_{+,-k}) \right\} \\ & + 2K \sum_k (\chi_{+,k}^\dagger \chi_{+,k} + \chi_{-,k}^\dagger \chi_{-,k}) \end{aligned} \quad (\text{S12})$$

$$\begin{aligned} & + \frac{4K}{N_z} \sum_{k,p,q} (\chi_{+,p}^\dagger \chi_{+,p+q} + \chi_{-,p}^\dagger \chi_{-,p+q}) (\psi_{+,k+q}^\dagger \psi_{+,k} + \psi_{-,k+q}^\dagger \psi_{-,k}) \\ & + \frac{4K}{N_z} \sum_{k,p,q} (\chi_{+,p}^\dagger \chi_{-,p+q} + \chi_{-,p}^\dagger \chi_{+,p+q}) (\psi_{+,k+q}^\dagger \psi_{-,k} + \psi_{-,k+q}^\dagger \psi_{+,k}), \\ H_{ZZ} = & -ig \sum_{k,q} \phi_q (\chi_{-k+q}^\dagger \psi_k^\dagger + \psi_k \chi_{-k-q}), \end{aligned} \quad (\text{S13})$$

where  $\epsilon_{\pm,k} \approx \pm v k_x$  and  $\Delta_{\pm,k} \approx -v k_y$  with  $v = 3Ka$ .

Considering two-component Dirac spinors of

$$\Psi_k = \begin{pmatrix} \psi_{+,k} \\ \psi_{-,-k}^\dagger \end{pmatrix}, \quad X_k = \begin{pmatrix} \chi_{+,k} \\ \chi_{-,-k}^\dagger \end{pmatrix}, \quad (\text{S14})$$

we reformulate the effective Hamiltonian as follows

$$H_K = \sum_k \Psi_k^\dagger (v k_x \tau^z + v k_y \tau^y) \Psi_k + 2K \sum_k X_k^\dagger \tau^z X_k + H_I, \quad (S15)$$

$$H_{ZZ} = -ig \sum_{k,q} \phi_q (X_{k+q}^\dagger \tau^x \Psi_k - \Psi_k^\dagger \tau^x X_{k-q}), \quad (S16)$$

where  $H_I$  represents four-fermion interactions between itinerant and localized fermions. It turns out that these effective interactions are not relevant in the renormalization group (RG) sense, which will be discussed below. Then, the effective action is given by

$$S = \int \frac{d^3k}{(2\pi)^3} \bar{\Psi}(k) i\gamma \cdot k \Psi(k) + \int \frac{d^3k}{(2\pi)^3} \bar{X}(k) (i\gamma_0 k_0 + i\gamma_1 M_X) X(k) + S_I - ig \int \frac{d^3k d^3q}{(2\pi)^6} (\bar{X}(k+q) \Psi(k) - \bar{\Psi}(k) X(k-q)) \phi(q), \quad (S17)$$

where  $\bar{\Psi}(k) = \Psi^\dagger(k) \gamma_0$  and  $\bar{X}(k) = X^\dagger(k) \gamma_0$ . Dirac gamma matrices are  $\gamma_0 = \sigma^x$ ,  $\gamma_1 = -\sigma^y$ , and  $\gamma_2 = \sigma^z$ .  $S_I$  is the action term corresponding to  $H_I$ . The excitation gap for the  $Z_2$ -flux fluctuations is  $M_X = 2K$  and the interaction strength between itinerant and localized fermionic spinons ( $S_I$ ) is  $4K$ . It is rather unexpected to see that the gap of localized spinon excitations appears with the  $\gamma_1$  matrix, which implies that  $M_X$  plays the role of an effective gauge field to generate the spinon current  $i\bar{X}(k) \gamma_1 X(k)$ .

It is natural to introduce an effective action  $S_\phi$  for the dynamics of zigzag AFM fluctuations into the above effective action, and  $S_\phi$  is given by

$$S_\phi = \frac{1}{2} \int \frac{d^3k}{(2\pi)^3} \phi(-k) (k^2 + r) \phi(k) + \frac{\lambda}{4!} \int \frac{d^3k d^3p d^3q}{(2\pi)^9} \phi(-k) \phi(k+q) \phi(-p-q) \phi(p). \quad (S18)$$

Here,  $r$  is an effective mass parameter and  $\lambda$  is an effective self-interaction constant. This  $\phi^4$ -theory is an effective field theory in an Ising AFM lattice model (10).

Through the  $g$ -vertex, critical fluctuations of the  $\phi$ -fields generate a kinetic term of the  $X$ -field. Including this kinetic term, we construct the partition function in an effective field theory as

$$Z_{eff} = \int D\Psi(k) DX(k) D\phi(k) \exp(-S_{eff}[\Psi(k), X(k), \phi(k)])$$

$$S_{eff}[\Psi(k), X(k), \phi(k)] = \int \frac{d^3k}{(2\pi)^3} \bar{\Psi}(k) i\gamma \cdot k \Psi(k) + \int \frac{d^3k}{(2\pi)^3} \bar{X}(k) i\gamma \cdot (k + M) X(k) - ig \int \frac{d^3k d^3q}{(2\pi)^6} \phi(q) (\bar{X}(k+q) \Psi(k) - \bar{\Psi}(k) X(k-q)) + \frac{1}{2} \int \frac{d^3k}{(2\pi)^3} \phi(-k) (k^2 + r) \phi(k) + \frac{\lambda}{4!} \int \frac{d^3k d^3p d^3q}{(2\pi)^9} \phi(-k) \phi(k+q) \phi(-p-q) \phi(p). \quad (S19)$$

Here, we neglect the four-fermion interaction term since it is irrelevant in RG sense (11). Also we set the velocities of two fields be identical because the Dirac theory recovers the Lorentz symmetry as it flows to the low-energy limit in RG (12). It is interesting to observe that the gapless point of being-itinerant spinons  $X(k)$  is separated from that of  $\Psi(k)$  in an amount of  $M = (0, M_X, 0)$  in the momentum space. This means that  $Z_2$  flux fluctuations driven by zigzag AFM excitations are represented by a current-flowing state in the Kitaev spin liquid phase.

## 2. Wilsonian renormalization group analysis

We rewrite the effective action in a  $D$ -dimension with a cutoff  $\Lambda$  as

$$\begin{aligned}
S = & \int_{\Lambda} \frac{d^D k}{(2\pi)^D} \bar{\Psi}(k) i\gamma \cdot k \Psi(k) + \int_{\Lambda} \frac{d^D k}{(2\pi)^D} \bar{X}(k) i\gamma \cdot (k + M) X(k) \\
& - ig \int_{\Lambda} \frac{d^D k d^D q}{(2\pi)^{2D}} (\bar{X}(k + q) \Psi(k) - \bar{\Psi}(k) X(k - q)) \phi(q) \\
& + \frac{1}{2} \int_{\Lambda} \frac{d^D k}{(2\pi)^D} k^2 \phi(-k) \phi(k) + \frac{\lambda}{4!} \int_{\Lambda} \frac{d^D k d^D p d^D q}{(2\pi)^{3D}} \phi(-k) \phi(k + q) \phi(-p - q) \phi(p).
\end{aligned} \tag{S20}$$

In order to perform the Wilsonian RG analysis, we separate all field variables into low and high energy-momentum parts

$$\begin{aligned}
\Psi(k) &= \Psi(k) \Theta \left[ k \left( \frac{\Lambda}{b} - k \right) \right] + \Psi(k) \Theta \left[ (\Lambda - k) \left( k - \frac{\Lambda}{b} \right) \right] \equiv \Psi_L(k) + \Psi_H(k), \\
X(k) &= X(k) \Theta \left[ k \left( \frac{\Lambda}{b} - k \right) \right] + X(k) \Theta \left[ (\Lambda - k) \left( k - \frac{\Lambda}{b} \right) \right] \equiv X_L(k) + X_H(k), \\
\phi(k) &= \phi(k) \Theta \left[ k \left( \frac{\Lambda}{b} - k \right) \right] + \phi(k) \Theta \left[ (\Lambda - k) \left( k - \frac{\Lambda}{b} \right) \right] \equiv \phi_L(k) + \phi_H(k).
\end{aligned} \tag{S21}$$

Here,  $k = \sqrt{\sum_{\mu=0}^d k_{\mu}^2}$  in the Euclidean signature and  $b$  is a scaling parameter to define the observation energy scale.  $\Theta(x)$  is a step function with  $\Theta(x) = 1$  for  $x \geq 0$  and  $\Theta(x) = 0$  for  $x < 0$ .

Implementing these expressions into the effective field theory and integrating over high energy degrees of freedom, i.e., performing the functional integral of  $\int D\Psi_H(k) D X_H(k) D \phi_H(k)$  in the perturbative way of the cumulant expansion, we obtain quantum-fluctuation corrections on the dynamics of low energy degrees of freedom. Both self-energy and vertex corrections can be absorbed into the original form of an effective action, introducing renormalization constants for the relation between unrenormalized and renormalized physical quantities (10). As the results, we find the renormalized field variables and constants as follows

$$\begin{aligned}
\Psi_R(k) &= b^{\Delta_{\Psi}} Z_{\Psi}^{-\frac{1}{2}} \Psi_L \left( \frac{k}{b} \right), \quad X_R(k) = b^{\Delta_X} Z_X^{-\frac{1}{2}} X_L \left( \frac{k}{b} \right), \quad \phi_R(k) = b^{\Delta_{\phi}} Z_{\phi}^{-\frac{1}{2}} \phi_L \left( \frac{k}{b} \right), \\
g_R &= b^{2 - \frac{D}{2}} Z_g^{-1} Z_{\Psi}^{\frac{1}{2}} Z_X^{\frac{1}{2}} Z_{\phi}^{\frac{1}{2}} g, \quad \lambda_R = b^{4-D} Z_{\lambda}^{-1} Z_{\phi}^2 \lambda, \quad M_R = b Z_M^{-1} Z_X M.
\end{aligned} \tag{S22}$$

Here the renormalized constants reflect effects of both self-energy and vertex corrections, and  $\Delta_{\Psi} = \Delta_X = -(D + 1)/2$ ,  $\Delta_{\phi} = -(D + 2)/2$  are mass dimensions of the fields. We also introduce not only the vertex renormalization constants of  $Z_g$  and  $Z_{\lambda}$  to include their vertex corrections but also the ‘mass’ renormalization constant of  $Z_M$  together with the wave-function renormalization constants such as  $Z_{\Psi}$ ,  $Z_X$ , and  $Z_{\phi}$  to absorb their self-energy corrections. As a result, we rewrite the effective field theory in terms of renormalized field variables and renormalized interaction-strength coefficients with rescaling of the energy-momentum space, which reproduces the original form of an effective field theory.

Now the ‘integral’ equations (S22) become translated into differential equations as follows

$$\begin{aligned}
\eta_{\Psi} &= \frac{1}{2} \frac{d \log Z_{\Psi}}{d \log b}, \quad \eta_X = \frac{1}{2} \frac{d \log Z_X}{d \log b}, \quad \eta_{\phi} = \frac{1}{2} \frac{d \log Z_{\phi}}{d \log b}, \\
\beta_g &\equiv \frac{d g_R}{d \log b} = g_R \left( 2 - \frac{D}{2} - \frac{d \log Z_g}{d \log b} + \eta_{\Psi} + \eta_X + \eta_{\phi} \right), \\
\beta_{\lambda} &\equiv \frac{d \lambda_R}{d \log b} = \lambda_R \left( 4 - D - \frac{d \log Z_{\lambda}}{d \log b} + 4 \eta_{\phi} \right).
\end{aligned} \tag{S23}$$

Here,  $\eta_{\Psi}$ ,  $\eta_X$ , and  $\eta_{\phi}$  represent anomalous scaling dimensions of each field variable, which results from correlated dynamics near quantum criticality.  $\beta_g$  and  $\beta_{\lambda}$  describe how each interaction parameter evolves as a function of an energy scale  $b$  self-consistently due to correlation effects. The initial condition of the effective field theory at  $\Lambda$  is defined as  $b = 1$  while  $b \rightarrow \infty$  gives rise to the low energy renormalization.

The functional integration for high energy degrees of freedom contributes self-energy corrections to low energy degrees of freedom

$$\begin{aligned}\Sigma_\Psi(k) &= g^2 \int_{\frac{\Lambda}{b}}^{\Lambda} \frac{d^D q}{(2\pi)^D} G_X(k+q) G_\phi(q), & \Sigma_X(k) &= g^2 \int_{\frac{\Lambda}{b}}^{\Lambda} \frac{d^D q}{(2\pi)^D} G_\Psi(k+q) G_\phi(q), \\ \Sigma_{\phi,1}(q) &= -2g^2 \int_{\frac{\Lambda}{b}}^{\Lambda} \frac{d^D k}{(2\pi)^D} \text{Tr} G_\Psi(k+q) G_X(k), & \Sigma_{\phi,2}(q) &= -\frac{\lambda}{2} \int_{\frac{\Lambda}{b}}^{\Lambda} \frac{d^D k}{(2\pi)^D} G_\phi(k),\end{aligned}\tag{S24}$$

as represented in the form of Feynman diagrams of Fig. S3. In this context, the three-point vertex with the coupling constant  $g$  contributes self-energy corrections to all excitations of  $\Psi(k)$ ,  $X(k)$ , and  $\phi(q)$  in the one-loop level. In addition, the self-interaction vertex with the coupling constant  $\lambda$  results in the self-energy correction on the Ising spin AFM fluctuations (14). Green's functions are given by

$$G_\Psi(k) = -\frac{i\gamma \cdot k}{k^2}, \quad G_X(k) = -\frac{i\gamma \cdot (k+M)}{(k+M)^2}, \quad G_\phi(k) = \frac{1}{k^2 + r}.\tag{S25}$$

The  $\Psi$ -propagator  $G_\Psi(k)$ ,  $X$ -propagator  $G_X(k)$ , and  $\phi$ -propagator  $G_\phi(k)$  are represented by a single line, double line, and dashed line, respectively, as shown in Fig. S3. Hereafter, we focus on the zigzag AFM quantum criticality at  $r = 0$ .

Such quantum fluctuations also affect the vertices and contribute corrections of

$$\begin{aligned}\Gamma_g &= -ig^3 \int_{\frac{\Lambda}{b}}^{\Lambda} \frac{d^D q}{(2\pi)^D} G_\phi(q) G_\Psi(q) G_X(q), \\ \Gamma_{\lambda,1} &= -\frac{3\lambda^3}{2} \int_{\frac{\Lambda}{b}}^{\Lambda} \frac{d^D q}{(2\pi)^D} [G_\phi(q)]^2, & \Gamma_{\lambda,2} &= g^4 \int_{\frac{\Lambda}{b}}^{\Lambda} \frac{d^D q}{(2\pi)^D} \text{Tr} G_X(q) G_\Psi(q) G_X(q) G_\Psi(q).\end{aligned}\tag{S26}$$

See Fig. S3 for Feynman diagrams. The three-point vertex is renormalized by itself in the one-loop level and also gives rise to the vertex renormalization for the four-point  $\lambda$ -vertex of the Ising spin fluctuations. The self-interaction vertex is also renormalized by itself in the one-loop level and its renormalization typically leads to the Wilson-Fisher fixed point (10). Here, we only consider most relevant interaction channels with zero energy-momentum transfer.

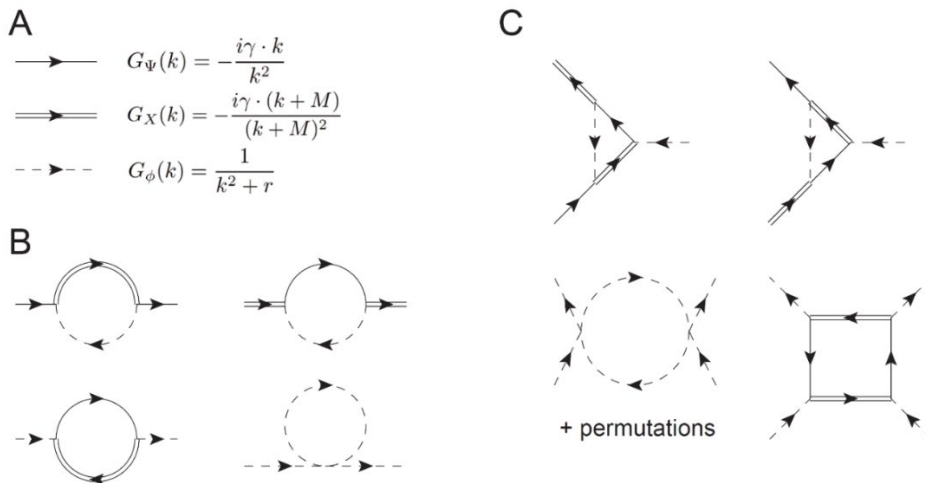

**Fig. S3 Feynman diagrams for self-energies and vertex corrections.** (A) The solid line, double line, and dashed line represent the  $\Psi$  propagator  $G_\Psi(k)$ ,  $X$  propagator  $G_X(k)$ , and  $\phi$  propagator  $G_\phi(k)$ , respectively. (B) The three-point interaction vertex with  $g$  contributes self-energy corrections to all excitations of  $\Psi(k)$ ,  $X(k)$ , and  $\phi(q)$  in the one-loop level. In addition, the self-interaction vertex with  $\lambda$  causes the mass renormalization, but does not the wave-function renormalization in the one-loop level. (C) The three-point (four-point or self-

interaction) vertex becomes renormalized by itself and additionally gives rise to the four-point vertex renormalization in the one-loop level.

In Appendix A, we describe all details of integrals for both self-energy and vertex corrections. Here we present all renormalization constants as follows

$$\begin{aligned}
Z_\Psi &= 1 - \frac{g_R^2}{2} S_D F_D^\Psi(M) \frac{dl}{\Lambda^{4-D}}, & Z_X &= 1 - \frac{g_R^2}{2} S_D \frac{dl}{\Lambda^{4-D}}, & Z_\phi &= 1 - g_R^2 S_D F_D^\phi(M) \frac{dl}{\Lambda^{4-D}}, \\
Z_g &= 1 + g_R^2 S_D G_D^g(M) \frac{dl}{\Lambda^{4-D}}, & Z_\lambda &= 1 + \frac{3\lambda_R}{2} S_D \frac{dl}{\Lambda^{4-D}} - 12 \frac{g_R^4}{\lambda_R} S_D G_D^\lambda(M) \frac{dl}{\Lambda^{4-D}}, \text{ and} \\
Z_M &= 1 + \frac{g_R^2}{2} S_D G_D^M(M) \frac{dl}{\Lambda^{4-D}},
\end{aligned} \tag{S27}$$

where  $S_D = \frac{2\pi^{D/2}}{(2\pi)^D \Gamma(D/2)}$  is the surface area of the  $D$ -dimensional sphere and the high energy-momentum domain is  $dl = \log b$ . The wave-function renormalization constant  $Z_\phi$  for the zigzag spin-fluctuation field  $\phi(k)$  originates from the three-point interaction vertex rather than the four-point self-interaction vertex in the one-loop level. Both three-point and four-point interaction vertices contribute to the four-point vertex renormalization constant in the one-loop level.

The mass dependent functions,  $F_D^{\Psi,\phi}(M)$  and  $G_D^{g,\lambda,M}(M)$  in the renormalization constants are as follows

$$\begin{aligned}
F_D^\Psi(M) &= \frac{2}{\sqrt{\pi}} \frac{\Gamma(\frac{D}{2})}{\Gamma(\frac{D-1}{2})} \int_0^1 ds \int_0^\pi d\phi \frac{(1-s)\sin^{D-2}\phi}{\left(1 + \frac{sM^2}{\Lambda^2} + \frac{2sM}{\Lambda} \cos\phi\right)^2}, \\
F_D^\phi(M) &= \frac{2}{\sqrt{\pi}} \frac{\Gamma(\frac{D}{2})}{\Gamma(\frac{D-1}{2})} \int_0^1 ds \int_0^\pi d\phi \sin^{D-2}\phi \frac{3s(1-s) + s^2(1-s)\frac{M^2}{\Lambda^2} + 2s(1-s^2)\frac{M}{\Lambda} \cos\phi}{\left(1 + \frac{sM^2}{\Lambda^2} + \frac{2sM}{\Lambda} \cos\phi\right)^2}, \\
G_D^g(M) &= \frac{2}{\sqrt{\pi}} \frac{\Gamma(\frac{D}{2})}{\Gamma(\frac{D-1}{2})} \int_0^1 ds \int_0^\pi d\phi \frac{(1-s)\sin^{D-2}\phi \left(1 + \frac{M}{\Lambda} \cos\phi\right)}{\left(1 + \frac{sM^2}{\Lambda^2} + \frac{2sM}{\Lambda} \cos\phi\right)^3}, \\
G_D^\lambda(M) &= \frac{2}{\sqrt{\pi}} \frac{\Gamma(\frac{D}{2})}{\Gamma(\frac{D-1}{2})} \int_0^1 ds \int_0^\pi d\phi s(1-s)\sin^{D-2}\phi \frac{1 + \frac{2M}{\Lambda} \cos\phi + \frac{2M^2}{\Lambda^2} \cos^2\phi - \frac{M^2}{\Lambda^2}}{\left(1 + \frac{sM^2}{\Lambda^2} + \frac{2sM}{\Lambda} \cos\phi\right)^4}, \text{ and} \\
G_D^M(M) &= \frac{2}{\sqrt{\pi}} \frac{\Gamma(\frac{D}{2})}{\Gamma(\frac{D-1}{2})} \int_0^1 ds \int_0^\pi d\phi \frac{\sin^{D-2}\phi}{\left(1 + \frac{sM^2}{\Lambda^2} + \frac{2sM}{\Lambda} \cos\phi\right)^2}.
\end{aligned} \tag{S28}$$

$F_D^\Psi(M)$  ( $F_D^\phi(M)$ ) results from the self-energy correction for  $\Psi$  spinons ( $\phi$  Ising spin fluctuations).  $G_D^g(M)$  and  $G_D^\lambda(M)$  come from quantum corrections for the three-point vertex with  $g$  and the self-interaction vertex with  $\lambda$ , respectively. Self-energies of the  $\Psi$  and  $X$  fields cause mass renormalization  $G_D^M(M)$ , which expands the difference between zero energy momentum points (the so-called Dirac points) of the  $\Psi$  and  $X$  fields.

Inserting the renormalization constants in Eq. (S27) into Eq. (S23), we derive the anomalous scaling dimensions

$$\begin{aligned}
\eta_\Psi &= \frac{1}{2} \frac{d \log Z_\Psi}{dl} = -\frac{g^2}{32\pi^2} F_4^\Psi(M), & \eta_X &= \frac{1}{2} \frac{d \log Z_X}{dl} = -\frac{g^2}{32\pi^2}, \\
\eta_\phi &= \frac{1}{2} \frac{d \log Z_\phi}{dl} = -\frac{g^2}{16\pi^2} F_4^\phi(M),
\end{aligned} \tag{S29}$$

and the  $\beta$ -functions

$$\beta_g = \frac{g}{2} - \frac{g^3}{16\pi^2} \left( 2G_4^g(M) + \frac{1}{2}F_4^\Psi(M) + F_4^\phi(M) + \frac{1}{2} \right), \quad \beta_\lambda = \lambda - \frac{3\lambda^2}{16\pi^2} + \frac{3g^4}{2\pi^2} G_4^\lambda(M). \quad (\text{S30})$$

Here we consider  $D = 4 - \epsilon$  with  $\epsilon = 1$  and obtain the mass dependent functions as follows

$$\begin{aligned} F_4^\Psi(M) &= \frac{4}{\pi} \int_0^1 ds \int_0^\pi d\phi \sin^2\phi \frac{1-s}{(1+sM^2+2sM\cos\phi)^2}, \\ F_4^\phi(M) &= \frac{4}{\pi} \int_0^1 ds \int_0^\pi d\phi \sin^2\phi \frac{3s(1-s) + s^2(1-s)M^2 + 2s(1-s^2)M\cos\phi}{(1+sM^2+2sM\cos\phi)^3}, \\ G_4^g(M) &= \frac{4}{\pi} \int_0^1 ds \int_0^\pi d\phi \sin^2\phi \frac{(1-s)(1+2M\cos\phi)}{(1+sM^2+2sM\cos\phi)^3}, \\ G_4^\lambda(M) &= \frac{4}{\pi} \int_0^1 ds \int_0^\pi d\phi s(1-s)\sin^2\phi \frac{1 + \frac{2M}{\Lambda}\cos\phi + \frac{2M^2}{\Lambda^2}\cos^2\phi - \frac{M^2}{\Lambda^2}}{\left(1 + \frac{sM^2}{\Lambda^2} + \frac{2sM}{\Lambda}\cos\phi\right)^4}. \end{aligned} \quad (\text{S31})$$

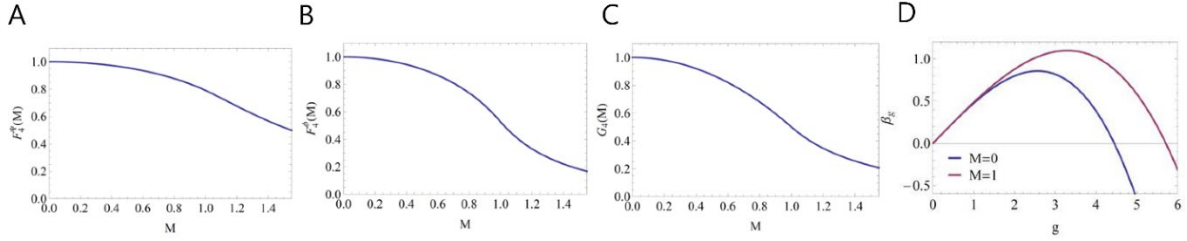

**Fig. S4** The functions  $F_4^\Psi(M)$ ,  $F_4^\phi(M)$ ,  $G_4^g(M)$  and the  $\beta$ -function  $\beta_g$ . We plot (A)  $F_4^\Psi(M)$ , (B)  $F_4^\phi(M)$ , and (C)  $G_4^g(M)$  as a function of  $M$ , respectively. (D)  $\beta_g$  in terms of  $g$  with  $M = 0$  (blue) and  $M = 1$  (magenta).

It is straightforward to solve the coupled  $\beta$ -functions (S30), and the interaction parameter  $g$  between spinon excitations and Ising spin fluctuations evolves to decouple from the self-interaction constant  $\lambda$ . The fixed point for the three-point interaction vertex is given by

$$\frac{g_*^2}{8\pi^2} = \left( 2G_4^g(M) + \frac{F_4^\Psi(M)}{2} + F_4^\phi(M) + \frac{1}{2} \right)^{-1}. \quad (\text{S32})$$

This interacting fixed point is stable as expected for the three-point interaction vertex in the abelian case. However, this effective interaction causes instability on the Wilson-Fisher fixed point, leading to a novel interacting fixed point

$$\lambda_* = \frac{\lambda_{WF} + \sqrt{\lambda_{WF}^2 + 32g_*^4 G_4^\lambda(M)}}{2}, \quad (\text{S33})$$

where  $\lambda_{WF} = 16\pi^2/3$  is the Wilson-Fisher fixed point. Figure S5 displays the flow diagram of the  $\beta$ -functions together with the new fixed point.

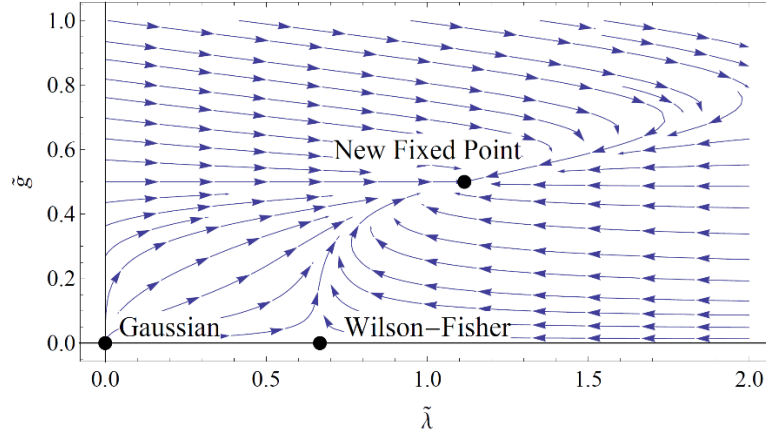

**Fig. S5 The renormalization group flow diagram of coupling constants.** Solving the coupled  $\beta$ -functions, we find RG flows in a  $\tilde{g} - \tilde{\lambda}$  coupling space with  $\tilde{g}^2 = g^2/8\pi^2$  and  $\tilde{\lambda} = \lambda/8\pi^2$ , and obtain a novel interacting fixed point.

Inserting this fixed-point value into Eq. (S29), we have

$$\begin{aligned}\eta_\Psi &= -\frac{F_4^\Psi(M)}{4\left(2G_4^g(M) + \frac{F_4^\Psi(M)}{2} + F_4^\phi(M) + \frac{1}{2}\right)}, \\ \eta_X &= -\frac{1}{4\left(2G_4^g(M) + \frac{F_4^\Psi(M)}{2} + F_4^\phi(M) + \frac{1}{2}\right)}, \\ \eta_\phi &= -\frac{F_4^\phi(M)}{2\left(2G_4^g(M) + \frac{F_4^\Psi(M)}{2} + F_4^\phi(M) + \frac{1}{2}\right)}.\end{aligned}\tag{S34}$$

It is interesting to observe that the Ising spin field  $\phi(k)$  acquires an anomalous scaling dimension in the one-loop level through interactions with spinon excitations. Meanwhile, without the three-point vertex, the anomalous scaling dimension requires the two-loop order at the Wilson-Fisher fixed point.

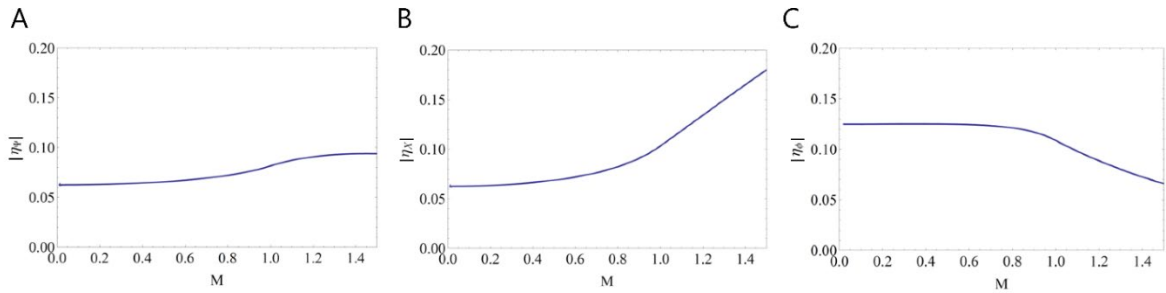

**Fig. S6 Anomalous scaling dimensions.** Anomalous scaling dimensions as a function of the  $Z_2$  flux gap  $M$  for (A)  $\eta_\Psi$ , (B)  $\eta_X$ , and (C)  $\eta_\phi$ .

### 3. Dynamic spin susceptibility

In order to extract the dynamical spin susceptibility at the  $\Gamma$ -point, we introduce a uniform field Zeeman coupling  $H_{UZ} = -g_u \sum_i \sigma_i^z H_i^u$ , which can be reformulated as

$$H_{UZ} = i g_u \int \frac{d^3 k d^3 q}{(2\pi)^6} H_u(q) (\bar{X}(k+q) \gamma_0 \Psi(k) - \bar{\Psi}(k) \gamma_0 X(k-q)). \quad (S35)$$

Here, we do not take into account for the coupling between the zigzag AFM  $\phi(k)$  and the uniform field since its effect is negligible in comparison with the ferro-component contribution of the  $\Gamma$ -point. Then, the spin susceptibility is given by

$$\chi_u(q) = \frac{1}{V} \frac{\delta^2 \ln Z_{eff}[H(q)]}{\delta H_u(-q) \delta H_u(q)} \Big|_{H(q)=0}, \quad (S36)$$

where  $Z_{eff}$  is the effective partition function including the Zeeman term. This 2<sup>nd</sup> derivative of the effective free energy with respect to the magnetic field reduces to the Kubo formula for the spin susceptibility as like

$$\begin{aligned} \chi_u(q) &= g_u^2 Z_{g_u}^2 Z_\Psi Z_X \frac{1}{V} \int_{k,k'} ((\bar{X}_R(k+q) \gamma_0 \Psi_R(k) \bar{\Psi}_R(k') \gamma_0 X_R(k'+q))_c \\ &\quad + (\bar{\Psi}_R(k) \gamma_0 X_R(k-q) \bar{X}_R(k'-q) \gamma_0 \Psi_R(k'))_c) \\ &= -g_u^2 Z_{g_u}^2 Z_\Psi Z_X \int_k \text{Tr} [\{G_X(k+q) + G_X(k-q)\} \gamma_0 G_\Psi(k) \gamma_0] \equiv g_u^2 Z_{g_u}^2 Z_\Psi Z_X \chi_R(q), \end{aligned} \quad (S37)$$

where  $Z_{g_u}$  is the renormalization constant for the effective coupling constant in the Zeeman term. The renormalization factors play roles of anomalous scaling dimensions in the spin susceptibility and account for the absence of well defined quasiparticle excitations near the interacting fixed point.

Inserting the spinon Green's functions into the above expression, we obtain  $\chi_R(q) \equiv \chi_\Gamma^{(0)}(iv, q)$  at finite temperatures,

$$\chi_\Gamma^{(0)}(iv, q) = -\frac{g_u^2}{\beta} \sum_{i\omega} \int \frac{d^2 k}{(2\pi)^2} \text{Tr} \left[ \frac{-i\gamma_0(\omega + \nu) - i\vec{\gamma} \cdot (\vec{k} + \vec{q} + \vec{M})}{(\omega + \nu)^2 + (\vec{k} + \vec{q} + \vec{M})^2} \gamma_0 \frac{-i\gamma_0 \omega - i\vec{\gamma} \cdot \vec{k}}{\omega^2 + k^2} \gamma_0 \right] + (q \rightarrow -q). \quad (S38)$$

After detailed calculations presented in Appendix B, we obtain  $\chi_\Gamma^{(0)}(iv, q)$  in a BCS (Bardeen-Cooper-Schrieffer) form with a coherence factor. Taking the analytic continuation for the frequency  $iv \rightarrow \nu + i\delta$ , we finally determine the imaginary part of the spin susceptibility  $\chi_u(q) \equiv \chi_\Gamma(iv, q)$  at the  $\Gamma$  point ( $\vec{q} \rightarrow 0$ ) as follows,

$$\begin{aligned} &\text{Im} \chi_\Gamma(\nu, q \rightarrow 0) \\ &= Z_{g_u}^2 Z_\Psi Z_X \begin{cases} \frac{g_u^2}{2\pi} \int_0^\pi d\theta \, k_0 \frac{\nu - 2k_0 - M \cos\theta}{\nu + M \cos\theta} \left( \tanh \frac{k_0}{2T} - \tanh \frac{k_0 - \nu}{2T} \right) & (\nu > M) \\ \frac{g_u^2}{2\pi} \int_{\pi-\theta_1}^\pi d\theta \, k_1 \frac{\nu + 2k_1 + M \cos\theta}{\nu - M \cos\theta} \left( \tanh \frac{k_1 + \nu}{2T} - \tanh \frac{k_1}{2T} \right) \\ \quad + \frac{g_u^2}{2\pi} \int_{\pi-\theta_2}^\pi d\theta \, k_2 \frac{\nu - 2k_2 - M \cos\theta}{\nu + M \cos\theta} \left( \tanh \frac{k_2}{2T} - \tanh \frac{k_2 - \nu}{2T} \right) & (\nu < M) \end{cases} \end{aligned}$$

where we used short-hand notations

$$\begin{aligned} k_0 &= \frac{1}{2} \frac{\nu^2 - M^2}{\nu + M \cos\theta}, & k_1 &= \frac{1}{2} \frac{M^2 - \nu^2}{\nu - M \cos\theta}, & k_2 &= \frac{1}{2} \frac{\nu^2 - M^2}{\nu + M \cos\theta} = k_0, \\ \cos\theta_1 &= \frac{\nu}{M}, & \cos\theta_2 &= -\frac{\nu}{M}. \end{aligned} \quad (S40)$$

In order to introduce anomalous scaling dimensions, we rewrite the renormalization constants as

$$Z_\Psi = 1 - \frac{g_R^2 S_D}{2\Lambda^{4-D}} F_D^\Psi(M) \ln b \approx e^{-\frac{g_R^2 S_D}{2\Lambda^{4-D}} F_D^\Psi(M) \ln b} = b^{-2\eta_\Psi}, \quad (S41)$$

$$Z_X = 1 - \frac{g_R^2 S_D}{2\Lambda^{4-D}} \ln b \approx e^{-\frac{g_R^2 S_D}{2\Lambda^{4-D}} \ln b} = b^{-2\eta_X}.$$

Here, we do not take into account the anomalous scaling of  $g_u$ , given by  $Z_{g_u}$  at the leading order. Then, we find the scaling theory for the spin susceptibility

$$\text{Im}\chi(\nu, M, T) = s^{1+2\eta_\Psi+2\eta_X} \text{Im}\chi\left(\frac{\nu}{s}, \frac{M}{s^{y_M}}, \frac{T}{s}\right) = T^{1+2\eta_\Psi+2\eta_X} \text{Im}\chi\left(\frac{\nu}{T}, \frac{M}{T^{y_M}}, 1\right), \quad (S42)$$

where we set  $s = T$  in the second equality and  $y_M$  is the scaling dimension of  $M$ . Assuming  $M/T^{y_M} \ll 1$ , we can expand  $\chi(\nu/T, M/T^{y_M}, 1)$  in  $M/T^{y_M}$ . Based on Eq. (S39), we find that the lowest non-vanishing term is  $(M/T^{y_M})^2$ . Accordingly, the spin susceptibility is given by

$$\text{Im}\chi(\nu, M, T) = \chi_0 T^{1+2\eta_\Psi+2\eta_X} (MT^{y_M})^2 \left(\frac{T}{\nu}\right)^{1-2\eta_\Psi-2\eta_X} \tanh \frac{\nu}{4T} \equiv T^{-\eta_X} f\left(\frac{\nu}{T}\right), \quad (S43)$$

where  $\chi_0$  is a cut-off dependent and non-universal constant. The anomalous scaling dimension of the spin susceptibility is  $\eta_X = 2y_M - (1 + 2\eta_\Psi + 2\eta_X)$  and the scaling function is  $f\left(\frac{\nu}{T}\right) = \chi_0 M^2 \left(\frac{T}{\nu}\right)^{1-2\eta_\Psi-2\eta_X} \tanh \frac{\nu}{4T}$ .

## B. Effective field theory, dynamic spin susceptibility, specific heat, and dynamical mean-field theory analysis for the low-energy strong-coupling fixed point

### 1. Effective field theory, dynamic spin susceptibility, and specific heat for the local quantum criticality

We start from an empirical formula for the spin susceptibility with an external magnetic field  $H$  (13)

$$\chi_{LQCP}(\omega, T, H) = \frac{A}{(aT - i\omega)^\alpha + a^\alpha T_N^\alpha}, \quad T_N = T_N(H=0)\delta h^{\nu_Z}. \quad (S44)$$

Here,  $\omega$  and  $T$  are frequency and temperature, respectively.  $T_N$  is the Néel temperature, and  $\delta h = 1 - H/H_c$ , where  $H_c$  is the critical field. The exponent  $\nu_Z \approx 0.125$  is experimentally determined from the specific heat data shown in Fig. 4(b) in the main text. Parameters  $A$ ,  $a$ , and  $\alpha$  can be obtained from fitting of the spin susceptibility data. The explicit form used in the fitting is the imaginary part of  $\chi_{LQCP}$  at the critical field,  $H = H_c$  so  $T_N = 0$ ;

$$\text{Im}\chi_{LQCP}(\omega, T, H_c) = \text{Im} \frac{A}{(aT - i\omega)^\alpha} = T^{-\alpha} \frac{A}{(a^2 T^2 + \omega^2)^{\alpha/2}} \sin\left(\alpha \tan^{-1} \frac{\omega}{aT}\right), \quad (S45)$$

which is Eq. (2) in the main text.

Based on this local form of the spin susceptibility, we write an effective action for the low-energy region as

$$Z = \int D\psi D\chi D\phi \ e^{-S[\psi, \chi, \phi]},$$

$$S[\psi, \chi, \phi] = \int_0^\beta d\tau \int d^2x \left[ \bar{\psi}(\tau, x) (\gamma^\tau \partial_\tau + v_\psi \gamma^i \partial_i) \psi(\tau, x) + \bar{\chi}(\tau, x) (\gamma^\tau \partial_\tau + i\gamma^i M_i) \psi(\tau, x) \right. \\ \left. - i\lambda \phi(\tau, x) (\bar{\chi}(\tau, x) \psi(\tau, x) - \bar{\psi}(\tau, x) \chi(\tau, x)) \right] \\ + \frac{1}{2} \int_0^\beta d\tau \int d^2x \phi(\tau, x) \chi_{LQCP}^{-1}(\tau - \tau') \phi(\tau', x). \quad (S46)$$

This expression looks quite similar to that for the description of high energy delocalized quantum criticality.

However, there exist two essential different aspects. Firstly, the spin dynamics is locally critical, described by  $\chi_{LQCP}^{-1}$  in the AFM spin-fluctuation part instead of the relativistic dispersion. In the Matsubara frequency space,  $\chi_{LQCP}^{-1}$  has the following form (14)

$$\chi_{LQCP}^{-1}(i\omega, T, H) = [(aT + |\omega|)^\alpha + a^\alpha T_N^\alpha]/A \quad (\text{S47})$$

assumed to be momentum independent based on both spectroscopy and specific heat results (experiments) as shown in the main text. Secondly, the dynamics of  $Z_2$  flux excitations is also local. Below, we perform the dynamical mean-field theory analysis in the non-crossing approximation (15, 16), which confirms that this renormalization ansatz is self-consistent.

Integrating over the  $\phi$ -field, we obtain the following effective action

$$\begin{aligned} Z &= \int D\psi D\chi \ e^{-S[\psi, \chi]}, \\ S[\psi, \chi] &= \frac{1}{2} \text{Tr} \log \chi_{LQCP}^{-1} \\ &+ \int_0^\beta d\tau \int d^2x \left[ \bar{\psi}(\tau, x) (\gamma^\tau \partial_\tau + v_\psi \gamma^i \partial_i) \psi(\tau, x) + \bar{\chi}(\tau, x) (\gamma^\tau \partial_\tau + i\gamma^i M_i) \psi(\tau, x) \right] \\ &- \frac{\lambda^2}{2} \int_0^\beta d\tau \int d^2x \int d^2x' \left[ \bar{\chi}(\tau, x) \psi(\tau, x) \chi_{LQCP}(\tau - \tau') \chi(\tau', x) \bar{\psi}(\tau', x) \right. \\ &\quad \left. + \bar{\psi}(\tau, x) \chi(\tau, x) \chi_{LQCP}(\tau - \tau') \psi(\tau', x) \bar{\chi}(\tau', x) \right]. \end{aligned} \quad (\text{S48})$$

Performing the self-consistent one-loop analysis in this effective field theory, we find that this effective field theory yields a fixed point, which is locally quantum critical, as a self-consistent solution. Here the pairing channel has been neglected for simplicity.

Based on this effective field theory, we calculate the free-energy

$$F = \frac{1}{2\beta} \text{Tr} \log \chi_{LQCP}^{-1}. \quad (\text{S49})$$

Here we neglect contributions of both fermions  $\psi$  and  $\chi$  since excitations at low temperatures are dominated by the AFM critical bosons. It is because the  $Z_2$  flux excitations are “gapped” and the itinerant Majorana fermions have the Dirac dispersion. Now the specific heat is

$$C_m(T) = -T \frac{\partial^2 F}{\partial T^2} = -\frac{T}{2\pi} \int_0^\infty dE \frac{\partial^2}{\partial T^2} \left( \coth \frac{E}{2T} \text{Im} \log \chi_{LQCP}^{-1} \right), \quad (\text{S50})$$

where

$$\text{Im} \log \chi_{LQCP}^{-1} = -\tan^{-1} \frac{(a^2 + x^2)^{\frac{\alpha}{2}} \sin \alpha \theta}{(a^2 + x^2)^{\frac{\alpha}{2}} \cos \alpha \theta + a^\alpha y^\alpha}, \quad x = \frac{E}{T}, \quad y = \frac{T_N}{T}, \quad (\text{S51})$$

and  $\theta = \tan^{-1} \frac{E}{aT}$ . From this analytic form, one can deduce Eq. (S51) as a function of  $T_N/T$ , or  $\delta h^{vz}/T$ . This scaling behavior originates from the local behavior of  $\chi_{LQCP}$ . Using the values  $\alpha \approx 0.30$  and  $a \approx 0.95$  obtained from fitting the dynamic spin susceptibility (Fig. 3(d) in the main text), the calculated specific heat is shown in Fig. S7.

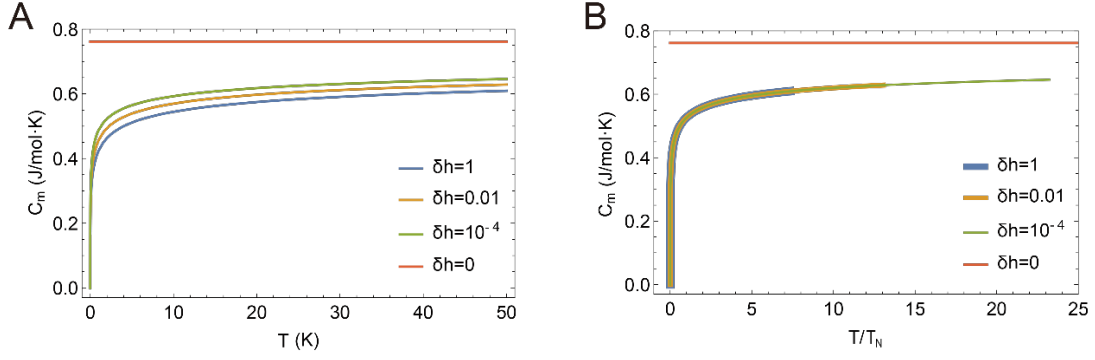

**Fig. S7 Calculated specific heat (A)** Specific heat  $C_m$  versus temperature  $T$  with various  $\delta h$ . **(B)** Scaling behavior of  $C_m$ . All curves with different  $\delta h$  collapse into a single curve. The value for the critical point ( $\delta h = 0$ ) corresponds to the value at  $T \rightarrow \infty$ .

Note that the parameter  $\alpha \approx 0.30$  is much smaller than  $\alpha = 1$  for the dynamics of a decoupled local moment. This critical exponent of the spin susceptibility could explain the plateau behavior of the specific heat in the intermediate temperature regime as shown in the main text. We show that this small value is supported by the self-consistent one-loop calculation in the next section. We also point out that the slow convergence to the critical value is due to the small value of  $\nu z \approx 0.125$ , which is not well understood within the first principle.

## 2. Dynamical mean-field theory analysis for the low-energy strong-coupling fixed point

One-loop self-energies for both  $\psi$  and  $\chi$  fermions are

$$\Sigma_\psi(i\omega, k) = -\frac{\lambda^2}{2\beta} \sum_{i\Omega} \int \frac{d^d q}{(2\pi)^d} \chi_{LQCP}(i\Omega) \mathcal{G}_\chi(i\omega - i\Omega, k - q), \quad (\text{S52})$$

$$\Sigma_\chi(i\omega, k) = -\frac{\lambda^2}{2\beta} \sum_{i\Omega} \int \frac{d^d q}{(2\pi)^d} \chi_{LQCP}(i\Omega) \mathcal{G}_\psi(i\omega - i\Omega, k - q), \quad (\text{S53})$$

where  $\mathcal{G}_\psi(i\omega, k)$  and  $\mathcal{G}_\chi(i\omega, k)$  are renormalized Green's functions of the  $\psi$ - and  $\chi$ -fields. These renormalized Green's functions satisfy the Dyson equations as follows

$$\mathcal{G}_\psi^{-1}(i\omega, k) = \mathcal{G}_\psi^{(0)-1}(i\omega, k) - \Sigma_\psi(i\omega, k) = \gamma^\tau (i\omega - \Sigma_{\psi,\tau}(i\omega, k)) + \gamma^i (iv_\psi k_i - \Sigma_{\psi,i}(i\omega, k)), \quad (\text{S54})$$

$$\mathcal{G}_\chi^{-1}(i\omega, k) = \mathcal{G}_\chi^{(0)-1}(i\omega, k) - \Sigma_\chi(i\omega, k) = \gamma^\tau (i\omega - \Sigma_{\chi,\tau}(i\omega, k)) + \gamma^i (iM_i - \Sigma_{\chi,i}(i\omega, k)). \quad (\text{S55})$$

Here,  $\mathcal{G}_\psi^{(0)}(i\omega, k) = [\gamma^\tau(i\omega) + \gamma^i(iv_\psi k_i)]^{-1}$  ( $\mathcal{G}_\chi^{(0)}(i\omega, k) = [\gamma^\tau(i\omega) + \gamma^i(iM_i)]^{-1}$ ) is the bare Green's function for the  $\psi$  ( $\chi$ ) fermion field.  $\Sigma_{\psi(\chi),\tau}(i\omega, k)$  and  $\Sigma_{\psi(\chi),i}(i\omega, k)$  are the temporal and spatial components of  $\Sigma_{\psi(\chi)}(i\omega, k)$ , respectively.

The last self-consistent condition is derived from the renormalized spin susceptibility. The spin susceptibility calculated with the renormalized Green's functions should be the same as  $\chi_{LQCP}(i\omega)$  from which we have started. Thus, the self-consistent condition is

$$\chi_{LQCP}(i\omega) = \frac{1}{\beta} \sum_{i\omega'} \int \frac{d^d k}{(2\pi)^d} \text{Tr} \mathcal{G}_\chi(i\omega', k) \mathcal{G}_\psi(i\omega' + i\omega, k + q). \quad (\text{S56})$$

Now we solve self-consistent equations formed by Eqs. (S52), (S53), and (S56). As discussed in the main text, we consider the power-law ansatz in frequency for the self-energy corrections,

$$\Sigma_\psi(i\omega, k) = \Sigma_\psi(i\omega) = C_\psi |\omega|^{\alpha_\psi}, \quad \Sigma_\chi(i\omega, k) = \Sigma_\chi(i\omega) = C_\chi |\omega|^{\alpha_\chi}. \quad (\text{S57})$$

Inserting these expressions into Eqs. (S52) and (S53) with the Dyson equations and the local spin susceptibility ansatz, we obtain

$$\gamma^\tau \Sigma_{\psi,\tau}(i\omega) + \gamma^i \Sigma_{\psi,i}(i\omega) = -\frac{\lambda^2}{2\beta} \sum_{i\Omega} \int \frac{d^d q}{(2\pi)^d} \left[ \frac{\chi_0}{(aT - i\Omega)^\alpha} \frac{\gamma^\tau(i\omega - i\Omega - \Sigma_{\chi,\tau}) - \gamma^i \Sigma_{\chi,i}}{(i\omega - i\Omega - \Sigma_{\chi,\tau})^2 + \Sigma_{\chi,i}^2} \right]_{i\omega - i\Omega}, \quad (\text{S58})$$

$$\begin{aligned} & \gamma^\tau \Sigma_{\chi,\tau}(i\omega) + \gamma^i \Sigma_{\chi,i}(i\omega) \\ &= -\frac{\lambda^2}{2\beta} \sum_{i\Omega} \int \frac{d^d q}{(2\pi)^d} \left[ \frac{\chi_0}{(aT - i\Omega)^\alpha} \frac{\gamma^\tau(i\omega - i\Omega - \Sigma_{\psi,\tau}) - \gamma^i(i v_\psi(k_i - q_i) - \Sigma_{\psi,i})}{(i\omega - i\Omega - \Sigma_{\psi,\tau})^2 + (i v_\psi(k_i - q_i) - \Sigma_{\psi,i})^2} \right]_{i\omega - i\Omega}. \end{aligned} \quad (\text{S59})$$

Performing the momentum integral in the second equation, we have

$$\Sigma_{\psi,\tau}(i\omega) = -\frac{\lambda^2}{2\beta} \sum_{i\Omega} \frac{\chi_0}{(aT - i\Omega)^\alpha} \frac{1}{i\omega - i\Omega - \Sigma_{\chi,\tau}(i\omega - i\Omega)}, \quad \Sigma_{\psi,i} = 0, \quad (\text{S60})$$

$$\begin{aligned} \Sigma_{\chi,\tau}(i\omega) &= -\frac{\lambda^2}{2\beta} \left( \frac{\pi}{2(i v_\psi)^d} \csc \frac{\pi d}{2} S_d \right) \sum_{i\Omega} \frac{\chi_0}{(aT - i\Omega)^\alpha} |i\omega - i\Omega - \Sigma_{\psi,\tau}(i\omega - i\Omega)|^{d-1}, \\ \Sigma_{\chi,i} &= 0. \end{aligned} \quad (\text{S61})$$

Substituting the power-law form of the self energies, we obtain their explicit expressions as follows

$$C_\psi |\omega|^{\alpha_\psi} = -\frac{\lambda^2}{2\beta} \sum_{i\Omega} \frac{\chi_0}{(aT - i\Omega)^\alpha} \frac{1}{i\omega - i\Omega - C_\chi |\omega - \Omega|^{\alpha_\chi}} \approx -\frac{\lambda^2}{2\beta} \sum_{i\Omega} \frac{\chi_0}{(aT - i\Omega)^\alpha} \frac{1}{C_\chi |\omega - \Omega|^{\alpha_\chi}}, \quad (\text{S62})$$

$$\begin{aligned} C_\chi |\omega|^{\alpha_\chi} &= -\frac{\lambda^2}{2\beta} \left( \frac{\pi}{2(i v_\psi)^d} \csc \frac{\pi d}{2} S_d \right) \sum_{i\Omega} \frac{\chi_0}{(aT - i\Omega)^\alpha} |i\omega - i\Omega - \Sigma_{\psi,\tau}(i\omega - i\Omega)|^{d-1} \\ &\approx -\frac{\lambda^2}{2\beta} \left( \frac{\pi}{2(i v_\psi)^d} \csc \frac{\pi d}{2} S_d \right) \sum_{i\Omega} \frac{\chi_0}{(aT - i\Omega)^\alpha} C_\psi^{d-1} |\omega - \Omega|^{(d-1)\alpha_\psi}. \end{aligned} \quad (\text{S63})$$

The self-consistent condition for the renormalized local susceptibility is

$$\begin{aligned} \chi_{LQCP}(i\omega) &= \frac{1}{\beta} \sum_{i\omega'} \int \frac{d^d k}{(2\pi)^d} \text{Tr} \mathcal{G}_\chi(i\omega', k) \mathcal{G}_\psi(i\omega' + i\omega, k + q) \\ &= \frac{2}{\beta} \sum_{i\omega'} \int \frac{d^d k}{(2\pi)^d} \frac{1}{i\omega' - \Sigma_{\chi,\tau}(i\omega')} \frac{i\omega' + i\omega - \Sigma_{\psi,\tau}(i\omega' + i\omega)}{(i\omega' + i\omega - \Sigma_{\psi,\tau}(i\omega' + i\omega))^2 + (i v_\psi k_i)^2}. \end{aligned} \quad (\text{S64})$$

Performing the momentum integral and substituting the power-law form of the self energies and the spin susceptibility, we have

$$\frac{\chi_0}{(aT - i\omega)^\alpha} \approx -\frac{2}{\beta} \left( \frac{\pi}{2(i v_\psi)^d} \csc \frac{\pi d}{2} S_d \right) \sum_{i\omega'} \frac{1}{C_\chi |\omega'|^{\alpha_\chi}} C_\psi^{d-1} |\omega' + \omega|^{(d-1)\alpha_\psi}. \quad (\text{S65})$$

To obtain the  $\omega/T$ -scaling, the power of  $T$  should be matched in Eqs. (S62), (S63), and (S65). As a result, we find the self-consistent condition for all the critical exponents of the power-law behaviors in frequency

$$\alpha_\psi = 1 - \alpha - \alpha_\chi, \quad \alpha_\chi = 1 - \alpha + (d-1)\alpha_\psi, \quad -\alpha = 1 - \alpha_\chi + (d-1)\alpha_\psi. \quad (\text{S66})$$

Solving these equations with  $d = 2$ , we obtain

$$\alpha_\psi = 0, \quad \alpha_\chi = 1, \quad \alpha = 0. \quad (\text{S67})$$

Indeed, these critical exponents cannot explain our experiments and the phenomenological analysis above.

However, this failure should be regarded as an artifact of the one-loop level analysis. The unitarity of this system has to give positive critical exponents for both  $\alpha_\psi$  and  $\alpha$  (17-19). If we introduce the flavor degeneracy  $N$  for both fermion excitations and take the large  $N$  limit as a theoretical device for a controllable approximation, the next leading order quantum corrections are in the order of  $1/N$ . It is beyond the scope of the present theoretical analysis to find such critical exponents with the introduction of vertex corrections. However, we claim that the appearance of  $1/N$  quantum corrections to the critical exponent  $\alpha$  supports why it is quite small compared to the dynamics of decoupled local magnetic moments. The present dynamical mean-field theory analysis at least confirms existence of the heavy-fermion-like local quantum criticality at low energies involving the emergent local dynamics of both  $Z_2$  flux and Ising AFM fluctuations.

## Appendix

### A. Self-energy and vertex corrections

The self-energy correction for the  $\Psi$ -field is given by

$$\begin{aligned}
\Sigma_\Psi(k) &= g^2 \int_{\frac{\Lambda}{b}}^{\Lambda} \frac{d^D q}{(2\pi)^D} \frac{1}{q^2} \frac{-i\gamma \cdot (k + q + M)}{(k + q + M)^2} \\
&= g^2 \int_{\frac{\Lambda}{b}}^{\Lambda} \frac{d^D q}{(2\pi)^D} \int_0^1 ds \frac{-i\gamma \cdot (k + q + M)}{[q + s(k + M)]^2} \\
&\approx g^2 \int_{\frac{\Lambda}{b}}^{\Lambda} \frac{d^D q}{(2\pi)^D} \int_0^1 ds \frac{-i\gamma \cdot [(1-s)k + M]}{(q + sM)^2} \\
&= -A_\Psi(g, M; \Lambda) i\gamma \cdot k - A_M(g, M; \Lambda) i\gamma \cdot M,
\end{aligned} \tag{SA1}$$

where the renormalization coefficients are

$$\begin{aligned}
A_\Psi(g, M; \Lambda) &= g^2 \frac{\pi^{\frac{D}{2}}}{(2\pi)^D \Gamma\left(\frac{D}{2}\right)} F_D^\Psi(M) \frac{dl}{\Lambda^{4-D}}, \\
F_D^\Psi(M) &= \frac{2}{\sqrt{\pi}} \frac{\Gamma\left(\frac{D}{2}\right)}{\Gamma\left(\frac{D-1}{2}\right)} \int_0^1 ds \int_0^\pi d\phi \frac{(1-s)\sin^{D-2}\phi}{\left(1 + \frac{sM^2}{\Lambda^2} + \frac{2sM}{\Lambda} \cos\phi\right)^2}, \\
A_M(g, M; \Lambda) &= g^2 \frac{\pi^{\frac{D}{2}}}{(2\pi)^D \Gamma\left(\frac{D}{2}\right)} G_D^M(M) \frac{dl}{\Lambda^{4-D}}, \\
G_D^M(M) &= \frac{2}{\sqrt{\pi}} \frac{\Gamma\left(\frac{D}{2}\right)}{\Gamma\left(\frac{D-1}{2}\right)} \int_0^1 ds \int_0^\pi d\phi \frac{\sin^{D-2}\phi}{\left(1 + \frac{sM^2}{\Lambda^2} + \frac{2sM}{\Lambda} \cos\phi\right)^2}.
\end{aligned} \tag{SA2}$$

Here, the generalized polar coordinate in a  $D$ -dimension has been used. We note that  $\delta\Lambda = \Lambda - \Lambda/b = \Lambda dl$ ,  $F_D^\Psi(M=0) = 1$ , and  $G_D^M(M=0) = 1$ .

Similarly, the self-energy correction for the  $X$ -field is given by

$$\Sigma_X(k) = g^2 \int_{\Lambda} \frac{d^D q}{(2\pi)^D} \frac{1}{q^2} \frac{-i\gamma \cdot (k + q)}{(k + q)^2} \approx -A_X(g, M; \Lambda) i\gamma \cdot k, \tag{SA3}$$

where the renormalization coefficient is

$$A_X(g, M; \Lambda) = g^2 \frac{\pi^{\frac{D}{2}}}{(2\pi)^D \Gamma\left(\frac{D}{2}\right)} \frac{dl}{\Lambda^{4-D}}. \tag{SA4}$$

Renormalization of  $M$ , the so-called mass renormalization, is irrelevant to  $\Sigma_X$  and is caused by  $\Sigma_\Psi$ . To show this renormalization, we introduce  $i\gamma \cdot M_\Psi$  in the  $\Psi$  sector. Then, the self-energy of the  $X$ -field is the same as that of the  $\Psi$ -field by replacing  $M$  with  $M_\Psi$ . Demanding  $M_{\Psi,ren} \equiv M_\Psi + \delta M_\Psi = 0$ , we have the renormalization as  $M \rightarrow M - A_M M$ .

The self-energy correction for the  $\phi$ -field is given by

$$\Sigma_\phi^{(1)} = -g^2 \int_{\frac{\Lambda}{b}}^{\Lambda} \frac{d^D q}{(2\pi)^D} \text{Tr} \left[ \frac{-i\gamma \cdot q - i\gamma \cdot (k + q + M)}{q^2 (k + q + M)^2} \right] = g^2 \int_{\frac{\Lambda}{b}}^{\Lambda} \frac{d^D q}{(2\pi)^D} \int_0^1 ds \frac{q \cdot (q + k + M)}{[q + s(k + M)]^2}. \quad (\text{SA5})$$

Expanding  $\Sigma_\phi^{(1)}(k)$  in terms of  $k^2$ , we have the field renormalization of the form  $-A_\phi(g, M; \Lambda) k^2$ , where

$$A_\phi(g, M; \Lambda) = g^2 \frac{\pi^{\frac{D}{2}}}{(2\pi)^D \Gamma\left(\frac{D}{2}\right)} \text{Tr} 1 F_D^\phi(M) \frac{dl}{\Lambda^{4-D}}, \quad (\text{SA6})$$

$$F_D^\phi(M) = \frac{2}{\sqrt{\pi}} \frac{\Gamma\left(\frac{D}{2}\right)}{\Gamma\left(\frac{D-1}{2}\right)} \int_0^1 ds \int_0^\pi d\phi \sin^{D-2}\phi \frac{3s(1-s) + s^2(1-s) \frac{M^2}{\Lambda^2} + 2s(1-s^2) \frac{M}{\Lambda} \cos\phi}{\left(1 + \frac{sM^2}{\Lambda^2} + \frac{2sM}{\Lambda} \cos\phi\right)^2}.$$

We note that  $F_D^\phi(M=0) = 1$ . The self-energy correction due to the  $\lambda$ -coupling effect is given by

$$\Sigma_\phi^{(2)} = -\lambda \int_{\frac{\Lambda}{b}}^{\Lambda} \frac{d^D q}{(2\pi)^D} \frac{1}{q^2}, \quad (\text{SA7})$$

which does not cause the field renormalization in this one-loop level.

The three-point vertex correction for the coupling constant  $g$  is given by

$$\Gamma_g(k, k + q, q) = ig^3 \int_{\frac{\Lambda}{b}}^{\Lambda} \frac{d^D q'}{(2\pi)^D} \frac{1}{q'^2} \frac{-i\gamma \cdot (k + q + q') - i\gamma \cdot (k + q' + M)}{(k + q + q')^2 (k + q' + M)^2}. \quad (\text{SA8})$$

Here, we set  $k = q = 0$  for all external momenta and perform the integral

$$\begin{aligned} \Gamma_g(0,0,0) &= ig^3 \int_{\frac{\Lambda}{b}}^{\Lambda} \frac{d^D q'}{(2\pi)^D} \frac{1}{q'^2} \frac{-i\gamma \cdot q' - i\gamma \cdot (q' + M)}{(q' + M)^2} \\ &= -2ig^3 \int_0^1 ds \int \frac{d^D q'}{(2\pi)^D} \frac{s(q'^2 + \gamma \cdot q' \cdot \gamma \cdot M)}{\{[q' + (1-s)M]^2 + s(1-s)M^2\}^3}. \end{aligned} \quad (\text{SA9})$$

For this  $\Gamma_g$  vertex correction, we have to consider a term proportional to the unit matrix in the spinor space. Taking into account  $\gamma_i \gamma_j \rightarrow \gamma_i \gamma_j$ , we obtain

$$\begin{aligned} \Gamma_g(0,0,0) &\rightarrow -2ig^3 \int_0^1 ds \int_{\frac{\Lambda}{b}}^{\Lambda} \frac{d^D q'}{(2\pi)^D} \frac{(1-s)(q'^2 + q' \cdot M)}{(q'^2 + 2sM \cdot q' + sM^2)^3} \\ &\approx -2ig^3 \frac{\pi^{\frac{D}{2}}}{(2\pi)^D \Gamma\left(\frac{D}{2}\right)} G_D^g(M) \frac{dl}{\Lambda^{4-D}}, \end{aligned} \quad (\text{SA10})$$

where the renormalization coefficient is

$$G_D^g(M) = \frac{2}{\sqrt{\pi}} \frac{\Gamma\left(\frac{D}{2}\right)}{\Gamma\left(\frac{D-1}{2}\right)} \int_0^1 ds \int_0^\pi d\phi \frac{(1-s) \sin^{D-2}\phi \left(1 + \frac{M}{\Lambda} \cos\phi\right)}{\left(1 + \frac{sM^2}{\Lambda^2} + \frac{2sM}{\Lambda} \cos\phi\right)^3}. \quad (\text{SA11})$$

We note that  $G_D^g(M=0) = 1$ .

The four-point vertex correction for the coupling constant  $\lambda$  is given by

$$\Gamma_\lambda^{(1)} = -\frac{3\lambda^2}{2} \int_{\frac{\Lambda}{b}}^{\Lambda} \frac{d^D q}{(2\pi)^D} \frac{1}{(q^2)^2} \approx -\frac{3\lambda^2}{2} \frac{2\pi^{\frac{D}{2}}}{(2\pi)^D \Gamma(\frac{D}{2})} \frac{dl}{\Lambda^{4-D}}, \quad (\text{SA12})$$

as well known (10).

The three-point interaction vertex gives rise to renormalization for the four-point self-interaction vertex as follows

$$\begin{aligned} \Gamma_\lambda^{(2)} &= 12g^4 \int_{\frac{\Lambda}{b}}^{\Lambda} \frac{d^D q}{(2\pi)^D} \text{Tr} \frac{-i\gamma \cdot (q+M) - i\gamma \cdot q}{(q+M)^2} \frac{i\gamma \cdot (q+M) - i\gamma \cdot q}{q^2} \\ &= 24g^4 \int_{\frac{\Lambda}{b}}^{\Lambda} \frac{d^D q}{(2\pi)^D} \frac{q^4 + 2(M \cdot q)q^2 + 2(M \cdot q)^2 - M^2 q^2}{q^4 (q+M)^4} \\ &= 24g^4 \int_0^1 ds \int_{\frac{\Lambda}{b}}^{\Lambda} \frac{d^D q}{(2\pi)^D} s(1-s) \frac{q^4 + 2(M \cdot q)q^2 + 2(M \cdot q)^2 - M^2 q^2}{(q^2 + sM^2 + 2sM \cdot q)^4} \\ &= 24g^4 \frac{2\pi^{\frac{D-1}{2}}}{(2\pi)^D \Gamma(\frac{D-1}{2})} \frac{dl}{\Lambda^{4-D}} \int_0^1 ds \int_0^\pi d\phi s(1-s) \sin^{D-2} \phi \frac{1 + \frac{2M}{\Lambda} \cos \phi + \frac{2M^2}{\Lambda^2} \cos^2 \phi - \frac{M^2}{\Lambda^2}}{\left(1 + \frac{sM^2}{\Lambda^2} + \frac{2sM}{\Lambda} \cos \phi\right)^4} \\ &= 24g^4 \frac{\pi^{\frac{D}{2}}}{(2\pi)^D \Gamma(\frac{D}{2})} G_D^\lambda(M) \frac{dl}{\Lambda^{4-D}}. \end{aligned} \quad (\text{SA13})$$

Here, we have

$$G_D^\lambda(M) = \frac{2}{\sqrt{\pi}} \frac{\Gamma(\frac{D}{2})}{\Gamma(\frac{D-1}{2})} \int_0^1 ds \int_0^\pi d\phi s(1-s) \sin^{D-2} \phi \frac{1 + \frac{2M}{\Lambda} \cos \phi + \frac{2M^2}{\Lambda^2} \cos^2 \phi - \frac{M^2}{\Lambda^2}}{\left(1 + \frac{sM^2}{\Lambda^2} + \frac{2sM}{\Lambda} \cos \phi\right)^4}. \quad (\text{SA14})$$

## B. Dynamic spin susceptibility

The  $\Gamma$ -point spin susceptibility is given by

$$\begin{aligned} \chi_\Gamma^{(0)}(iv, q) &= -\frac{1}{\beta} \sum_{i\omega} \int \frac{d^2 k}{(2\pi)^2} \text{Tr} \left[ \frac{-i\gamma_0(\omega + v) - i\vec{\gamma} \cdot (\vec{k} + \vec{q} + \vec{M})}{(\omega + v)^2 + (\vec{k} + \vec{q} + \vec{M})^2} \gamma_0 \frac{-i\gamma_0 \omega - i\gamma \cdot k}{\omega^2 + k^2} \gamma_0 \right] \\ &\quad + (q \rightarrow -q) \\ &= -\frac{2}{\beta} \sum_{i\omega} \int \frac{d^2 k}{(2\pi)^2} \frac{i\omega(i\omega + iv) + \vec{k} \cdot (\vec{k} + \vec{q} + \vec{M})}{[(i\omega)^2 - \vec{k}^2][(i\omega + iv)^2 - (\vec{k} + \vec{q} + \vec{M})^2]} + (q \rightarrow -q). \end{aligned} \quad (\text{SA15})$$

Performing the Matsubara frequency summation, we obtain

$$\begin{aligned} &-\frac{1}{\beta} \sum_{i\omega} \frac{i\omega(i\omega + iv) + \vec{k} \cdot (\vec{k} + \vec{q} + \vec{M})}{[(i\omega)^2 - \vec{k}^2][(i\omega + iv)^2 - (\vec{k} + \vec{q} + \vec{M})^2]} \\ &= -\frac{1}{4} \left( 1 + \frac{\vec{k} \cdot (\vec{k} + \vec{q} + \vec{M})}{|\vec{k}| |\vec{k} + \vec{q} + \vec{M}|} \right) \left[ \frac{f(|\vec{k}|) - f(|\vec{k} + \vec{q} + \vec{M}|)}{iv + |\vec{k}| - |\vec{k} + \vec{q} + \vec{M}|} + \frac{f(-|\vec{k}|) - f(-|\vec{k} + \vec{q} + \vec{M}|)}{iv - |\vec{k}| + |\vec{k} + \vec{q} + \vec{M}|} \right] \\ &\quad -\frac{1}{4} \left( 1 - \frac{\vec{k} \cdot (\vec{k} + \vec{q} + \vec{M})}{|\vec{k}| |\vec{k} + \vec{q} + \vec{M}|} \right) \left[ \frac{f(|\vec{k}|) - f(-|\vec{k} + \vec{q} + \vec{M}|)}{iv + |\vec{k}| + |\vec{k} + \vec{q} + \vec{M}|} + \frac{f(-|\vec{k}|) - f(|\vec{k} + \vec{q} + \vec{M}|)}{iv - |\vec{k}| - |\vec{k} + \vec{q} + \vec{M}|} \right]. \end{aligned} \quad (\text{SA16})$$

As a result, we find

$$\begin{aligned}
\chi_{\Gamma}^{(0)}(iv, q) = & -\frac{1}{2} \int \frac{d^2 k}{(2\pi)^2} \left( 1 + \frac{\vec{k} \cdot (\vec{k} + \vec{q} + \vec{M})}{|\vec{k}| |\vec{k} + \vec{q} + \vec{M}|} \right) \left[ \frac{f(|\vec{k}|) - f(|\vec{k} + \vec{q} + \vec{M}|)}{iv + |\vec{k}| - |\vec{k} + \vec{q} + \vec{M}|} \right. \\
& \left. + \frac{f(-|\vec{k}|) - f(-|\vec{k} + \vec{q} + \vec{M}|)}{iv - |\vec{k}| + |\vec{k} + \vec{q} + \vec{M}|} \right] \\
& - \frac{1}{2} \int \frac{d^2 k}{(2\pi)^2} \left( 1 - \frac{\vec{k} \cdot (\vec{k} + \vec{q} + \vec{M})}{|\vec{k}| |\vec{k} + \vec{q} + \vec{M}|} \right) \left[ \frac{f(|\vec{k}|) - f(-|\vec{k} + \vec{q} + \vec{M}|)}{iv + |\vec{k}| + |\vec{k} + \vec{q} + \vec{M}|} \right. \\
& \left. + \frac{f(-|\vec{k}|) - f(|\vec{k} + \vec{q} + \vec{M}|)}{iv - |\vec{k}| - |\vec{k} + \vec{q} + \vec{M}|} \right] + (q \rightarrow -q).
\end{aligned} \tag{SA17}$$

Taking into account  $iv \rightarrow v + i\delta$  and the limit of  $q \rightarrow 0$ , we obtain

$$\begin{aligned}
\chi_{\Gamma}^{ret, (0)}(v, \vec{q} = 0) \\
= & -\frac{1}{4\pi^2} \int_0^\infty dk \int_0^{2\pi} d\theta \ k \left( 1 + \frac{k + M \cos \theta}{k_M} \right) \left[ \frac{f(k) - f(k_M)}{v + k - k_M + i\delta} + \frac{f(-k) - f(-k_M)}{v - k + k_M + i\delta} \right] \\
& - \frac{1}{4\pi^2} \int_0^\infty dk \int_0^{2\pi} d\theta \ k \left( 1 - \frac{k + M \cos \theta}{k_M} \right) \left[ \frac{f(k) - f(-k_M)}{v + k + k_M + i\delta} + \frac{f(-k) - f(k_M)}{v - k - k_M + i\delta} \right],
\end{aligned} \tag{SA18}$$

where the short-hand notation is  $k_M = \sqrt{k^2 + M^2 + 2Mk \cos \theta}$ .

It is straightforward to extract out the imaginary part

$$\begin{aligned}
\text{Im} \chi_{\Gamma}^{ret, (0)}(v, \vec{q} = 0) \\
= & \frac{1}{4\pi} \int_0^\infty dk \int_0^{2\pi} d\theta \ k \left( 1 + \frac{k + M \cos \theta}{k_M} \right) [f(k) - f(k_M)] \delta(v + k - k_M) \\
& + \frac{1}{4\pi} \int_0^\infty dk \int_0^{2\pi} d\theta \ k \left( 1 + \frac{k + M \cos \theta}{k_M} \right) [f(-k) - f(-k_M)] \delta(v - k + k_M) \\
& + \frac{1}{4\pi} \int_0^\infty dk \int_0^{2\pi} d\theta \ k \left( 1 - \frac{k + M \cos \theta}{k_M} \right) [f(k) - f(-k_M)] \delta(v + k + k_M) \\
& + \frac{1}{4\pi} \int_0^\infty dk \int_0^{2\pi} d\theta \ k \left( 1 - \frac{k + M \cos \theta}{k_M} \right) [f(-k) - f(k_M)] \delta(v - k - k_M).
\end{aligned} \tag{SA19}$$

Without any loss of generality, we consider  $v > 0$ . Then, we have

$$\begin{aligned}
\text{Im} \chi_{\Gamma}^{ret, (0)}(v, \vec{q} = 0) \\
= & \frac{1}{2\pi} \int_0^\infty dk \int_0^\pi d\theta \ k \frac{v + 2k + M \cos \theta}{v + k} [f(k) - f(k + v)] \delta(v + k - k_M) \\
& + \frac{1}{2\pi} \int_0^\infty dk \int_0^\pi d\theta \ k \frac{v - 2k - M \cos \theta}{v - k} [f(-k) - f(-k + v)] \delta(v - k + k_M) \\
& + \frac{1}{2\pi} \int_0^\infty dk \int_0^\pi d\theta \ k \frac{v - 2k - M \cos \theta}{v - k} [f(-k) - f(-k + v)] \delta(v - k - k_M).
\end{aligned} \tag{SA20}$$

First, we consider  $v > M$ . Then, the first and the second delta functions are zero. As a result, we find

$$\begin{aligned} \text{Im}\chi_{\Gamma}^{ret,(0)}(\nu, \vec{q} = 0) \\ = \frac{1}{2\pi} \int_0^{\infty} dk \int_0^{\pi} d\theta \ k \frac{\nu - 2k - M\cos\theta}{\nu - k} [f(-k) - f(-k + \nu)] \delta(\nu - k - k_M). \end{aligned} \quad (\text{SA21})$$

Performing the  $\theta$ -integration, we obtain

$$\text{Im}\chi_{\Gamma}^{ret,(0)}(\nu, \vec{q} = 0) = \frac{1}{4\pi} \int_{\nu-M}^{\nu+M} dk \sqrt{\frac{M^2 - (2k - \nu)^2}{\nu^2 - M^2}} \left( \tanh \frac{k}{2T} - \tanh \frac{k - \nu}{2T} \right). \quad (\text{SA22})$$

Second, we consider  $\nu < M$ . Then, the third delta function is zero. As a result, we find

$$\begin{aligned} \text{Im}\chi_{\Gamma}^{ret,(0)}(\nu, \vec{q} = 0) \\ = \frac{1}{2\pi} \int_{M-\nu}^{\infty} dk \frac{\nu + 2k + M\cos\theta_1}{M\sin\theta_1} [f(k) - f(k + \nu)] \\ + \frac{1}{2\pi} \int_{M+\nu}^{\infty} dk \frac{-\nu + 2k + M\cos\theta_2}{M\sin\theta_2} [f(-k) - f(-k + \nu)] \end{aligned} \quad (\text{SA23})$$

$$\begin{aligned} = \frac{1}{4\pi} \int_{M-\nu}^{\infty} dk \sqrt{\frac{(2k + \nu)^2 - M^2}{M^2 - \nu^2}} \left( \tanh \frac{k + \nu}{2T} - \tanh \frac{k}{2T} \right) \\ + \frac{1}{4\pi} \int_{M+\nu}^{\infty} dk \sqrt{\frac{(2k - \nu)^2 - M^2}{M^2 - \nu^2}} \left( \tanh \frac{k}{2T} - \tanh \frac{k - \nu}{2T} \right), \end{aligned}$$

where  $\cos\theta_1 = \frac{(\nu+k)^2 - M^2 - k^2}{2Mk}$  and  $\cos\theta_2 = \frac{(\nu-k)^2 - M^2 - k^2}{2Mk} = \cos\theta_0$ .

## References and Notes

1. A. Kitaev, Anyons in an exactly solved model and beyond. *Annals of Physics* **321**, 2-111 (2006).
2. H. B. Cao *et al.*, Low-temperature crystal and magnetic structure of  $\alpha$ -RuCl<sub>3</sub>. *Phys. Rev. B* **93**, 134423 (2016).
3. R. D. Johnson *et al.*, Monoclinic crystal structure of  $\alpha$ -RuCl<sub>3</sub> and the zigzag antiferromagnetic ground state. *Phys. Rev. B* **92**, 235119 (2015).
4. S.-Y. Park *et al.*, Emergence of the Isotropic Kitaev Honeycomb Lattice with Two-dimensional Ising Universality in  $\alpha$ -RuCl<sub>3</sub>. *arXiv:1609.05690* (2016).
5. K. Ran *et al.*, Spin-Wave Excitations Evidencing the Kitaev Interaction in Single Crystalline  $\alpha$ -RuCl<sub>3</sub>. *Phys. Rev. Lett.* **118**, 107203 (2017).
6. H.-D. Chen, Z. Nussinov, Exact results of the Kitaev model on a hexagonal lattice: spin states, string and brane correlators, and anyonic excitations. *J. Phys. A: Math. Theor.* **41**, 075001 (2008).
7. D.-H. Lee, G.-M. Zhang, T. Xiang, Edge Solitons of Topological Insulators and Fractionalized Quasiparticles in Two Dimensions. *Phys. Rev. Lett.* **99**, 196805 (2007).
8. A. O. Gogolin, A. A. Nersisyan, A. M. Tsvelik, *Bosonization and strongly correlated systems*. (Cambridge University Press, 1998).
9. J. R. Schrieffer, *Theory of superconductivity*. (Perseus Books, Reading, Mass., 1999).
10. J. Zinn-Justin, *Quantum field theory and critical phenomena*. (Clarendon Press, New York, Oxford, New York, 4<sup>th</sup> ed., 2002).
11. K. G. Wilson, Quantum Field - Theory Models in Less Than 4 Dimensions. *Phys. Rev. D* **7**, 2911 (1973).
12. J. González, F. Guinea, M. A. H. Vozmediano, Non-Fermi liquid behavior of electrons in the half-filled honeycomb lattice (A renormalization group approach). *Nucl. Phys. B* **424**, 595-618 (1994).
13. A. Schröder *et al.*, Onset of antiferromagnetism in heavy-fermion metals. *Nature* **407**, 351-355 (2000).
14. N. Nagaosa, *Quantum Field Theory in Strongly Correlated Electron Systems*. (Springer, 1999).
15. O. Parcollet, A. Georges, G. Kotliar, A. Sengupta, Overscreened multichannel SU(N) Kondo model: Large-N solution and conformal field theory. *Phys. Rev. B* **58**, 3794 (1998).
16. E. Müller-Hartmann, Self-consistent perturbation theory of the anderson model: Ground state properties. *Z. Phys. B* **57**, 281 (1984).
17. S. Ferrara, A. Grillo, R. Gatto, G. Parisi, Analyticity properties and asymptotic expansions of conformal covariant green's functions. *Il Nuovo Cimento A* **19**, 667-695 (1974).
18. S. Minwalla, Restrictions imposed by superconformal invariance on quantum field theories. *Adv. Theor. Math. Phys.* **2**, 783-851 (1998).
19. D. Poland, S. Rychkov, A. Vichi, The conformal bootstrap: Theory, numerical techniques, and applications. *Rev. Mod. Phys.* **91**, 015002 (2019).
